# Supplementary material for: HiFi-123: Towards High-fidelity One Image to 3D Content Generation
Source: arXiv:2310.06744 source file (2024-07-12)
Supplement: Supplementary file 1 [file SDEdit.tex]

\begin{figure}[t]
  \centering
  \includegraphics[width=1.\textwidth]{images/ablate_sdedit.pdf}
  \caption{Novel view enhancement results of SDEdit.}
  % \vspace{-1em}
\label{fig:sdedit}
\end{figure}
