# Supplementary material for: HiFi-123: Towards High-fidelity One Image to 3D Content Generation
Source: arXiv:2310.06744 source file (2024-07-12)
Supplement: Supplementary file 3 [file ablate_nvs.tex]

\begin{figure*}[t]
  \centering
  \includegraphics[width=.9\textwidth]{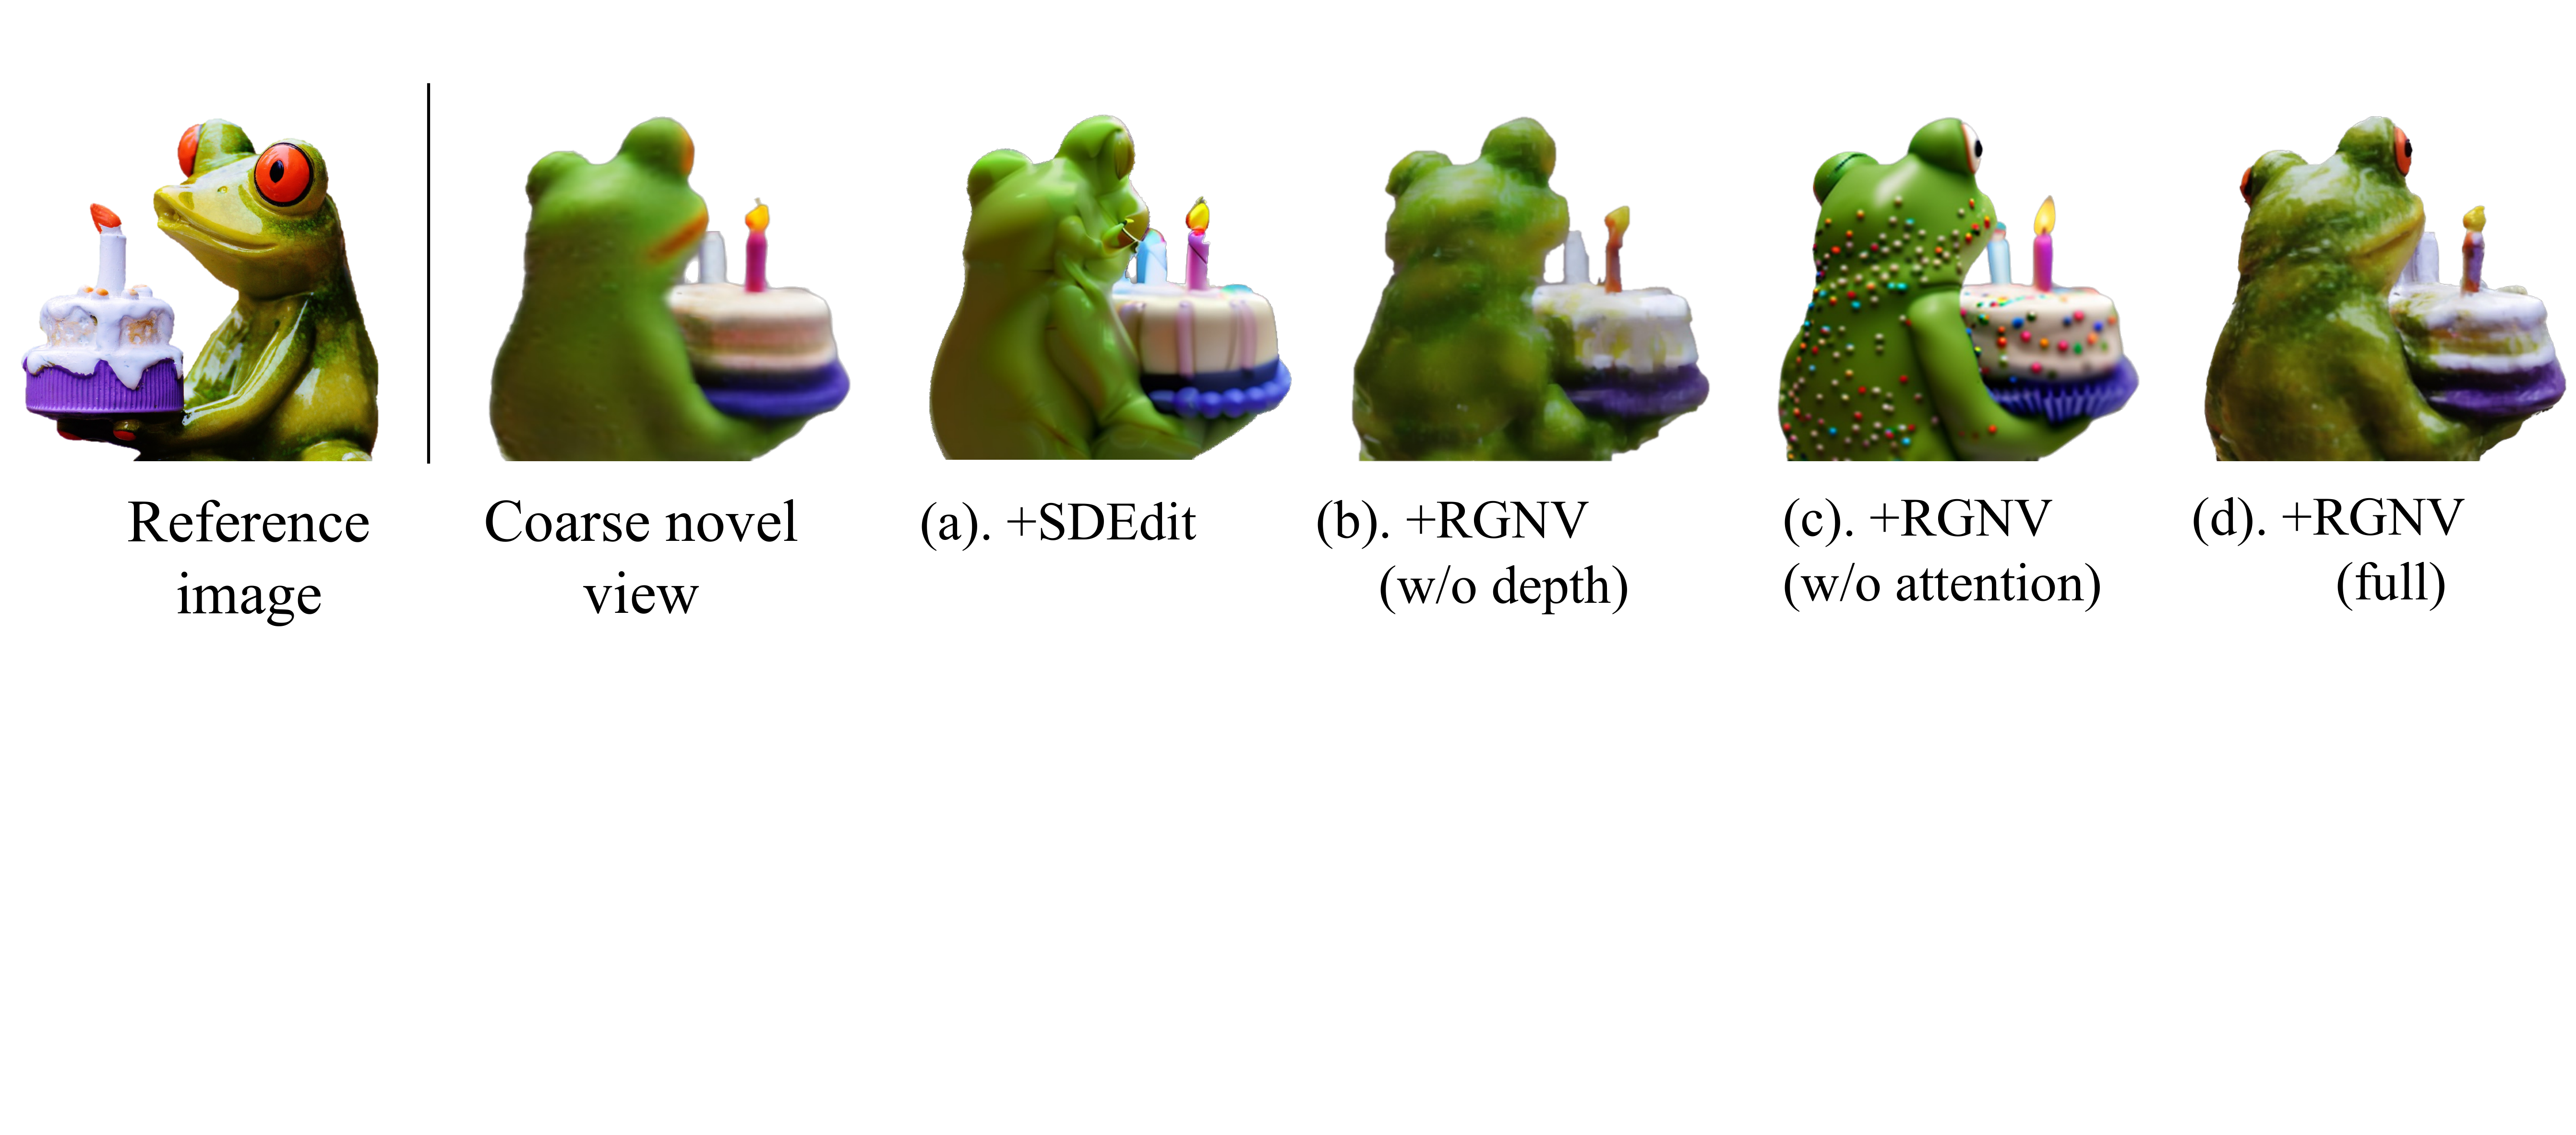}
  \caption{Ablation on novel view enhancement. We validate the effectiveness of using depth-based DDIM inversion and attention injection.}
  % \vspace{-1em}
\label{fig:ablate_nvs}
\end{figure*}
