# Supplementary material for: HiFi-123: Towards High-fidelity One Image to 3D Content Generation
Source: arXiv:2310.06744 source file (2024-07-12)
Supplement: Supplementary file 5 [file comp_zero123.tex]

\begin{figure*}[t]
  \centering
  \includegraphics[width=.8\textwidth]{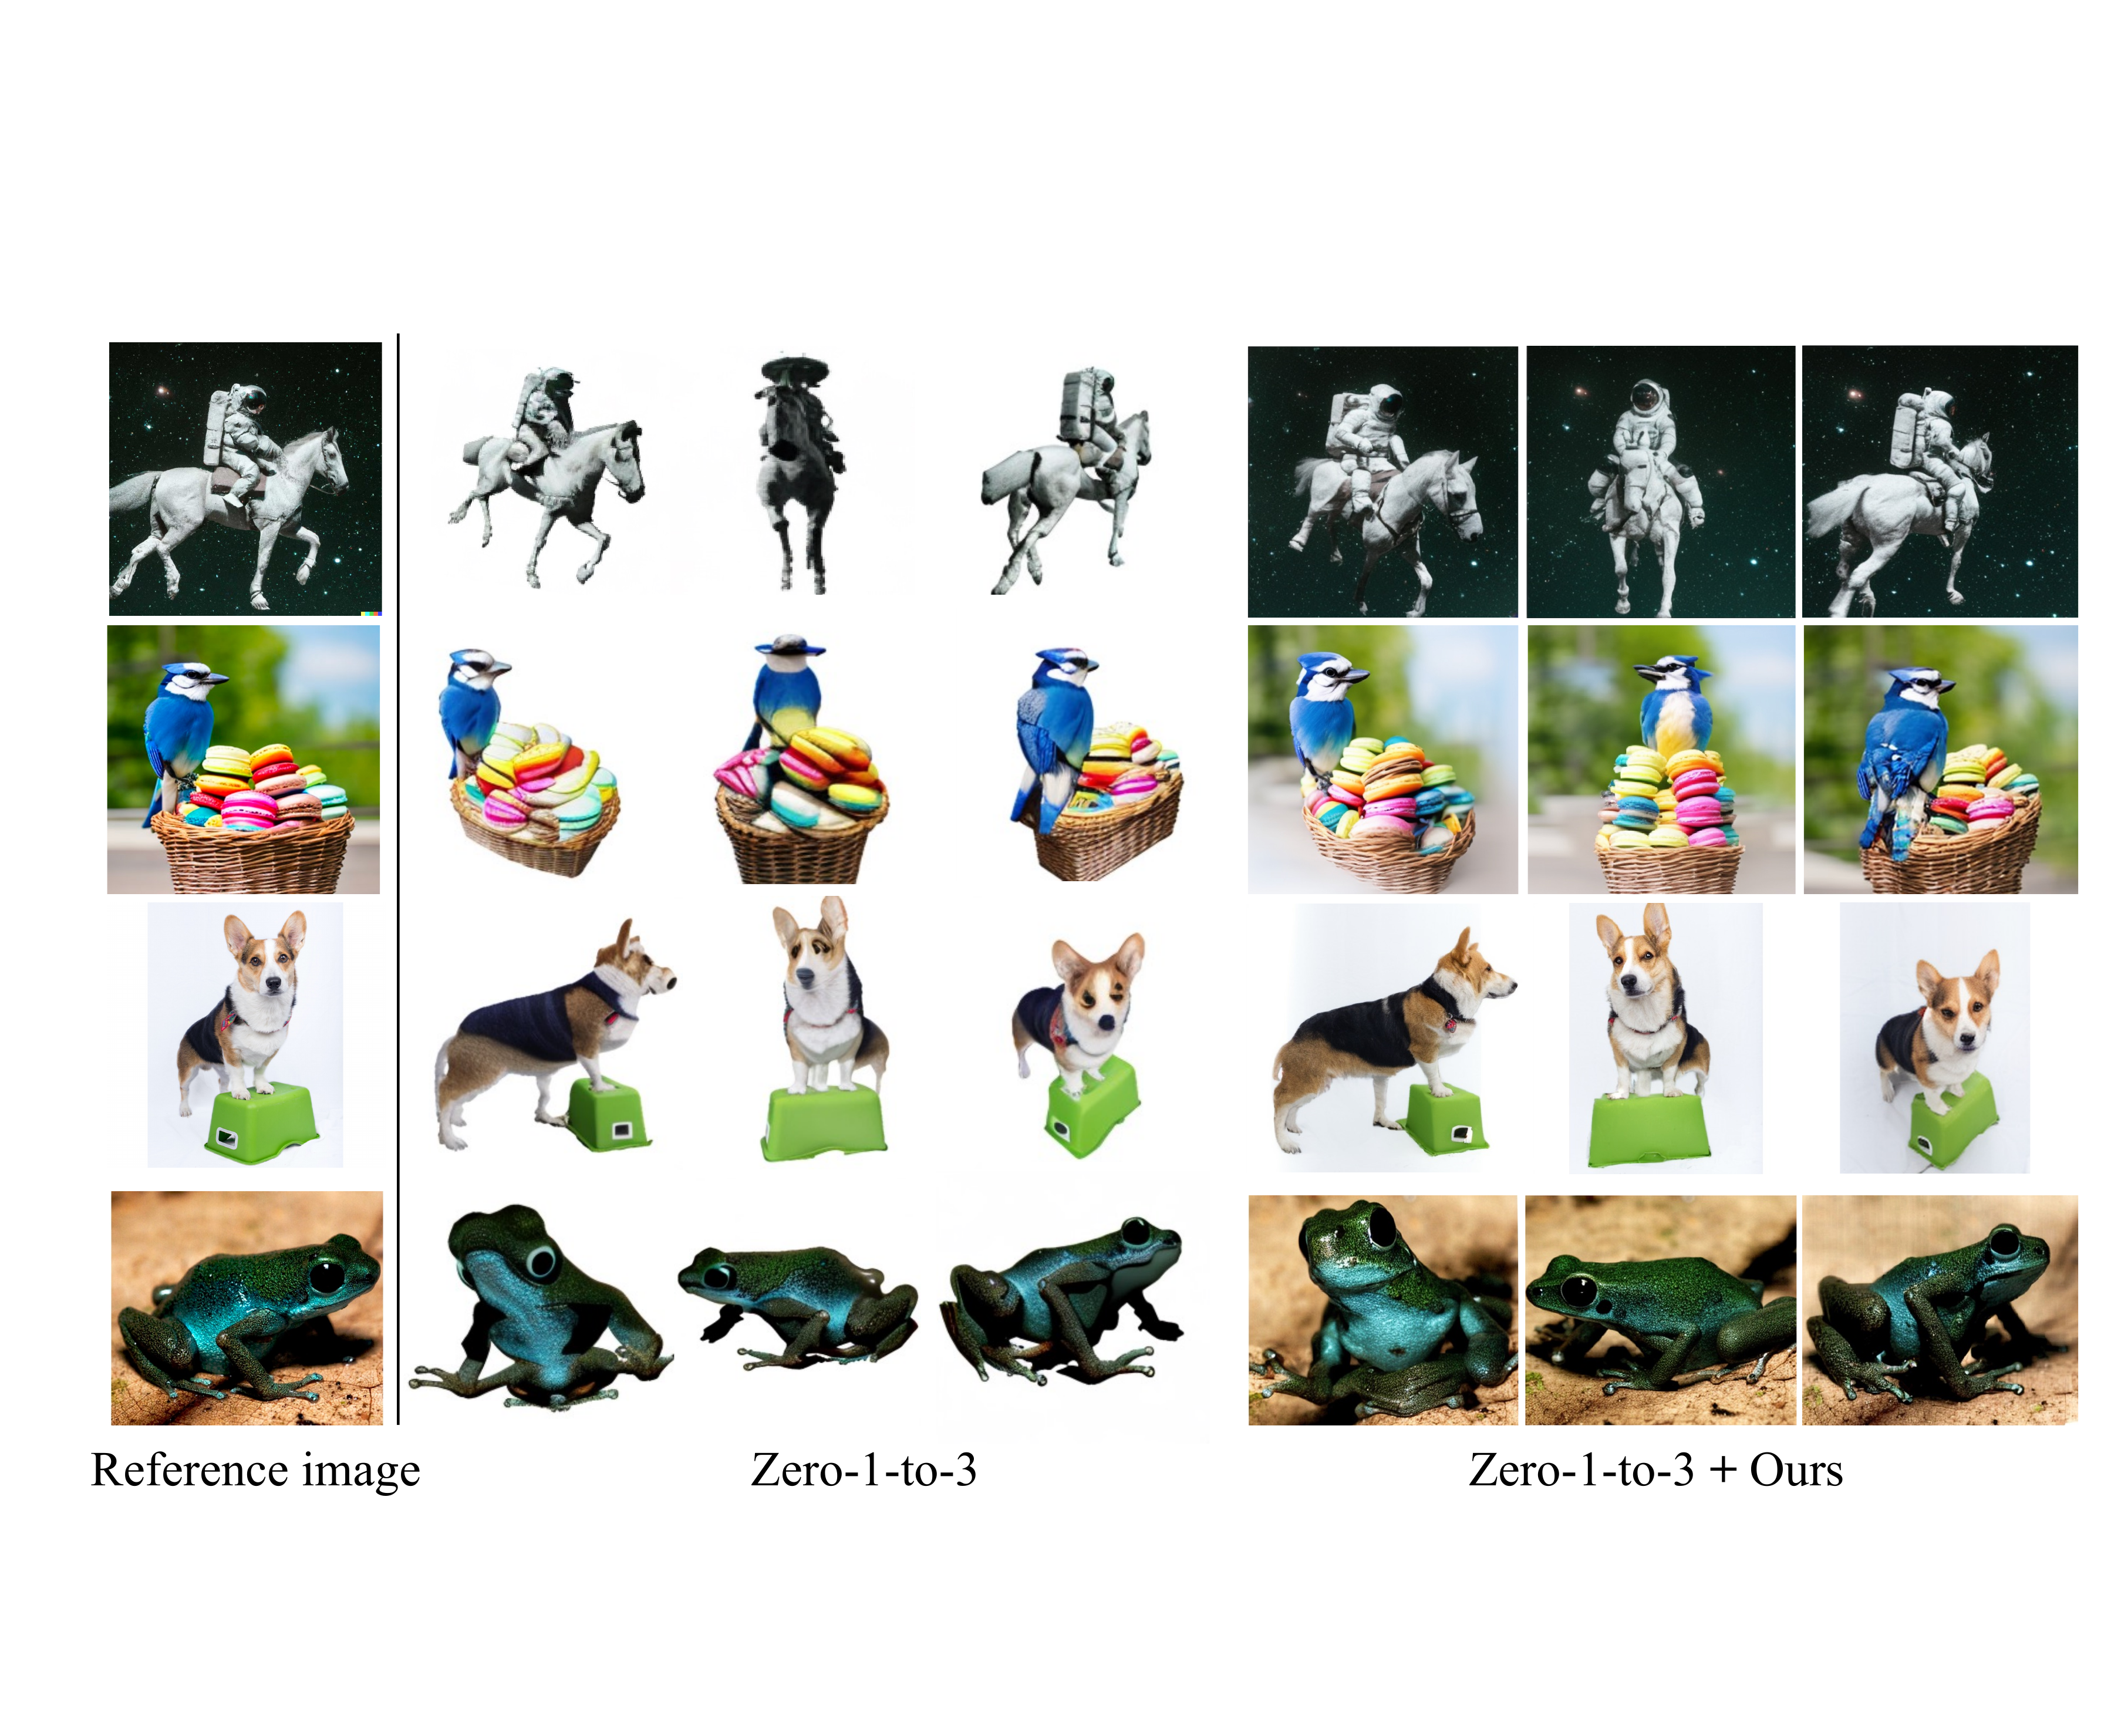}
  \vspace{-1em}
  \caption{Qualitative comparison with Zero-1-to-3 on zero-shot novel view synthesis. It can be found that our method can generate novel views with higher fidelity and finer texture details.}
  \vspace{-1em}
\label{fig:comp_zero123}
\end{figure*}
