# Supplementary material for: HiFi-123: Towards High-fidelity One Image to 3D Content Generation
Source: arXiv:2310.06744 source file (2024-07-12)
Supplement: Supplementary file 6 [file more.tex]

\begin{figure*}[t]
  \centering
  \includegraphics[width=.88\textwidth]{images/more_results.pdf}
  \caption{Qualitative results of the coarse stage and refine stage produced by our image-to-3D generation method. It can be observed that although the coarse stage can provide a reasonable geometry, its texture details are significantly different from the reference image. Through optimization in the refine stage, the texture quality is effectively improved.}
  % \vspace{-2em}
\label{fig:more}
\end{figure*}
