# Supplementary material for: HiFi-123: Towards High-fidelity One Image to 3D Content Generation
Source: arXiv:2310.06744 source file (2024-07-12)
Supplement: Supplementary file 7 [file pipeline.tex]

\begin{figure}[t]
  \centering
  \includegraphics[width=0.47\textwidth]{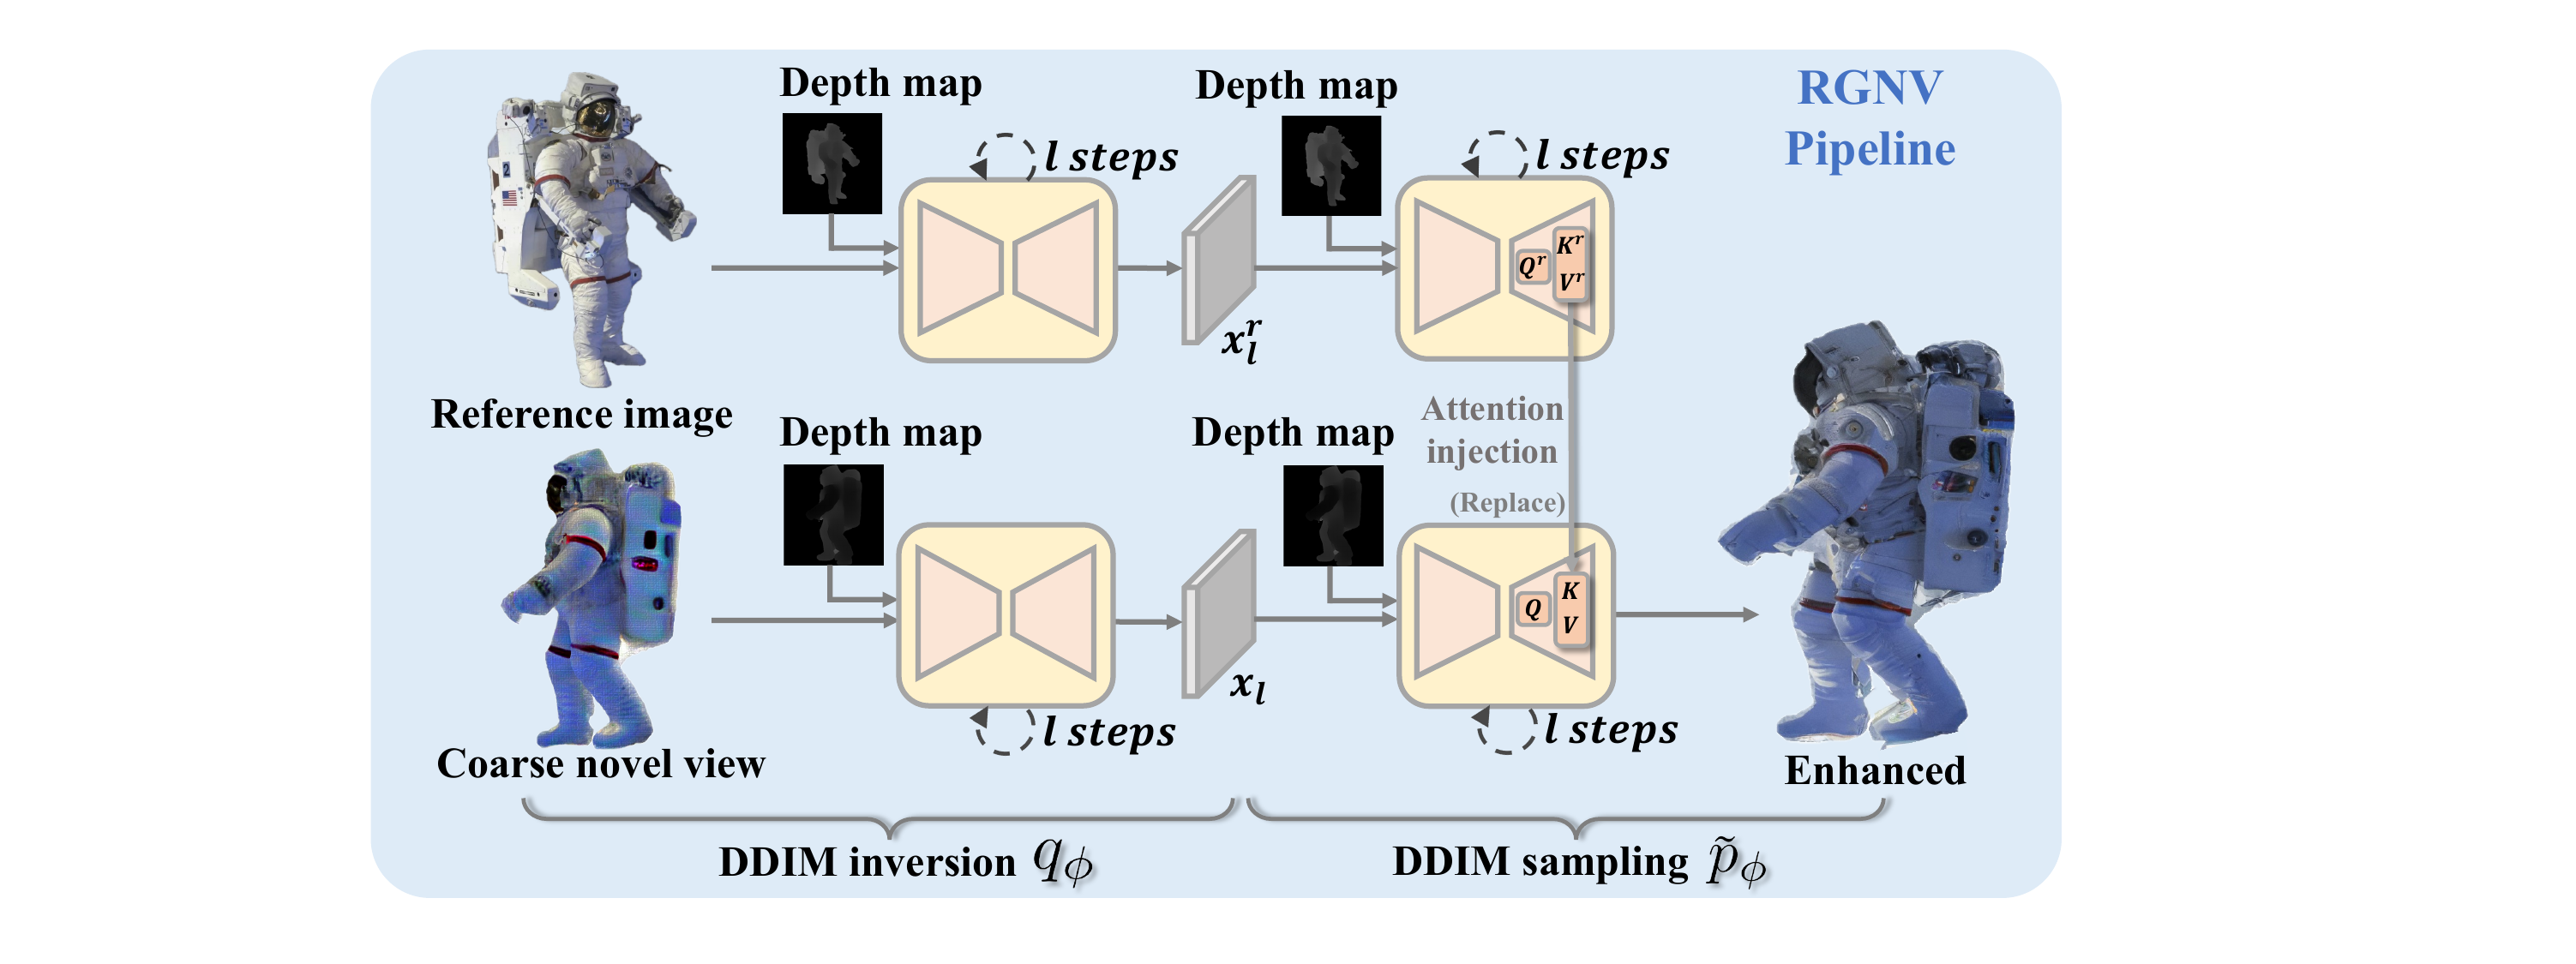}
  \caption{Reference-guided novel view enhancement pipeline. Our pipeline performs depth-based DDIM inversion and sampling on both the reference image and coarse novel view, and utilizes attention injection to transfer detail textures from the reference image to the coarse novel view.}
  % \vspace{-1em}
\label{pipeline}
\end{figure}
