# Supplementary material for: HiFi-123: Towards High-fidelity One Image to 3D Content Generation
Source: arXiv:2310.06744 source file (2024-07-12)
Supplement: Supplementary file 10 [file i23_gso.tex]

\begin{table}[t]
\centering
    \resizebox{0.9\linewidth}{!}{
  \begin{tabular}{l|ccccc}
\toprule
 & PSNR$\uparrow$ & SSIM$\uparrow$ & LPIPS$\downarrow$ & CD$\downarrow$ & IoU$\uparrow$\\ \midrule
Make-it-3D~\cite{tang2023make}& 22.38 & 0.734 & 0.251 & 0.086 & 0.368  \\
Magic123~\cite{qian2023magic123}& 30.16 & \textbf{0.789} & 0.237 & 0.066 & 0.461 \\
Ours& \textbf{32.05} & 0.785 & \textbf{0.221} & \textbf{0.055} & \textbf{0.493}\\
\bottomrule
\end{tabular}}
  \caption{Quantitative comparison with image-to-3D generation baselines on GSO dataset.}
  \label{tab:gso_i23}
  \vspace{-1.5em}
\end{table}
