# Supplementary material for: HiFi-123: Towards High-fidelity One Image to 3D Content Generation
Source: arXiv:2310.06744 source file (2024-07-12)
Supplement: Supplementary file 11 [file i23_single.tex]

%   \captionof{table}{Quantitative comparison with image-to-3D generation baselines.}
%   \label{tab:i23}
%   \resizebox{\linewidth}{!}{
% \begin{tabular}{l|ccc}
% \toprule
%  & LPIPS$\downarrow$  & Contextual$\downarrow$ & CLIP$\uparrow$ \\ \midrule
% RealFusion& 0.35 & 2.18& 0.81 \\
% Make-It-3D & 0.23 & 1.97& 0.90\\
% Magic123& \textbf{0.19} & 1.88 & 0.88  \\
% Ours& 0.21 & \textbf{1.63} & \textbf{0.92} \\
% \bottomrule
% \end{tabular}
%   }

\begin{table}[t]
\centering
  \resizebox{0.6\linewidth}{!}{
\begin{tabular}{l|ccc}
\toprule
 & LPIPS$\downarrow$  & Contextual$\downarrow$ & CLIP$\uparrow$ \\ \midrule
RealFusion~\cite{melas2023realfusion}& 0.35 & 2.18& 0.81 \\
Make-It-3D~\cite{tang2023make} & 0.23 & 1.97& 0.90\\
Magic123~\cite{qian2023magic123}& \textbf{0.19} & 1.88 & 0.88  \\
Ours& 0.21 & \textbf{1.63} & \textbf{0.92} \\
\bottomrule
\end{tabular}}
  \caption{Quantitative comparison with image-to-3D generation baselines on single view dataset.}
  \label{tab:single_i23}
  \vspace{-1.5em}
\end{table}
