# Supplementary material for: HiFi-123: Towards High-fidelity One Image to 3D Content Generation
Source: arXiv:2310.06744 source file (2024-07-12)
Supplement: Supplementary file 12 [file refine_gso.tex]

\begin{table}[t]
\centering
    \resizebox{0.71\linewidth}{!}{
  \begin{tabular}{l|ccc}
\toprule
 & PSNR$\uparrow$ & SSIM$\uparrow$ & LPIPS$\downarrow$ \\ \midrule
Coarse& 23.74 & 0.726 & 0.259   \\
Refine(SDS)& 26.43 & 0.757 & 0.240  \\
Refine(RGSD)& \textbf{32.05} & \textbf{0.785} & \textbf{0.221} \\
\bottomrule
\end{tabular}}
  \caption{Refine stage ablation on GSO~\cite{downs2022google} dataset. We compare the results of coarse stage, refine stage using SDS loss and refine stage using RGSD loss. The results demonstrate the effectiveness of refine stage training using RGSD loss.}
  \label{tab:refine_gso}
  \vspace{-1.5em}
\end{table}
