# Supplementary material for: HiFi-123: Towards High-fidelity One Image to 3D Content Generation
Source: arXiv:2310.06744 source file (2024-07-12)
Supplement: Supplementary file 13 [file refine_single.tex]

\begin{table}[t]
\centering
  \resizebox{0.66\linewidth}{!}{
\begin{tabular}{l|cc}
\toprule
 & Contextual$\downarrow$ & CLIP$\uparrow$ \\ \midrule
Coarse& 1.90 & 0.83 \\
Refine(SDS) & 1.93 & 0.86\\
Refine(RGSD) & \textbf{1.63} & \textbf{0.92} \\
\bottomrule
\end{tabular}}
  \caption{Refine stage ablation on single view dataset. We compare the results of coarse stage, refine stage using SDS loss and refine stage using RGSD loss. The results demonstrate the effectiveness of refine stage training using RGSD loss.}
  \label{tab:refine_single}
\end{table}
