# Supplementary material for: HiFi-123: Towards High-fidelity One Image to 3D Content Generation
Source: arXiv:2310.06744 source file (2024-07-12)
Supplement: Supplementary file 14 [file zero_metrics.tex]

\setlength{\tabcolsep}{2pt}
\begin{figure}[t]
% \begin{minipage}[c]{0.470\linewidth}
%   \centering
%   \captionof{table}{Quantitative comparison with image-to-3D generation baselines.}
%   \label{tab:i23}
%   \resizebox{\linewidth}{!}{
% \begin{tabular}{l|ccc}
% \toprule
%  & LPIPS$\downarrow$  & Contextual$\downarrow$ & CLIP$\uparrow$ \\ \midrule
% RealFusion& 0.35 & 2.18& 0.81 \\
% Make-It-3D & 0.23 & 1.97& 0.90\\
% Magic123& \textbf{0.19} & 1.88 & 0.88  \\
% Ours& 0.21 & \textbf{1.63} & \textbf{0.92} \\
% \bottomrule
% \end{tabular}
%   }
% \end{minipage}\hfill
\begin{minipage}[c]{0.45\linewidth}
  \centering
  \resizebox{\linewidth}{!}{
\begin{tabular}{l|ccc}
\toprule
 & Contextual$\downarrow$ & CLIP$\uparrow$ \\ \midrule
Zero-1-to-3~\cite{liu2023zero}& 1.94 & 0.89  \\
Ours& \textbf{1.60} & \textbf{0.93} \\
\bottomrule
\end{tabular}}
  \captionof{table}{Quantitative comparison with Zero-1-to-3 on single view dataset.}
  \label{tab:zero_single}

\end{minipage}\hfill
\begin{minipage}[c]{0.5\linewidth}
  \centering
  \resizebox{\linewidth}{!}{
\begin{tabular}{l|ccc}
\toprule
 & PSNR$\uparrow$  & SSIM$\uparrow$ & LPIPS$\downarrow$ \\ \midrule
Zero-1-to-3~\cite{liu2023zero}& 34.58 & 0.763 & 0.231  \\
Ours& \textbf{36.89} & \textbf{0.795} & \textbf{0.214} \\
\bottomrule
\end{tabular}}
  \captionof{table}{Quantitative comparison with Zero-1-to-3 on GSO dataset.}
  \label{tab:zero_3D}

\end{minipage}\hfill
% \vspace{-1em}
\end{figure}
